# Supplementary material for: SF2SE3: Clustering Scene Flow into SE(3)-Motions via Proposal and Selection
Source: arXiv:2209.08532 source file (2022-09-26)
Supplement: Supplementary file 1 [file main.tex]

\newpage

\section{Appendix}

\subsection{Gaussian Inlier Probability}
To calculate the inlier probabilities, we define the inlier probability for a single Gaussian random variable as follows
\begin{gather}
    \label{eq:gauss_inlier_prob}
    P_{I, Gauss.}(a, \mu, \sigma^2) = 2 (1 - F( \mu + |a|, \mu, \sigma^2)) \in [0, 1].
\end{gather}
This is illustrated in Figure \ref{fig:inlier_probab}.
\begin{figure}
    \centering
    \includesvg[scale=0.3]{chapters/3_approach/figures/inlier_probability.svg}
    \caption{On the left side is depicted in blue the probability density function $f(x)$ for a Gaussian distribution with $\mu=0$ and $\sigma^2=1$. The red area indicates the the Gaussian Inlier Probability $P_{I,Gauss}(a=1)$. On the right side, the resulting inlier probabilities are visualized, where the y-axis is shared with the left diagram.}
    \label{fig:inlier_probab}
\end{figure}

\subsection{Results Odometry for Individual Sequences}

In addition to the overall results for odometry in the main paper, we provide results for individual sequences of the TUM RGB-D dataset in Table \ref{tab:eval_odo_rep_seq}. 
\begin{table}[]
\centering
\caption{Odometry evaluation for individual sequences of the TUM RGB-D dataset based on the relative pose error. For comparison the results of the two-frame based solutions RigidMask \cite{yang2021learning_rigidmask}, VO-SF \cite{jaimez2017fast} and of the model-based solutions RGBD-SLAM-Dyn \cite{dai2020rgb}, ORB-SLAM2 \cite{mur2017orb} are reported.}
\label{tab:eval_odo_rep_seq}
%\begin{adjustbox}{totalheight=\textheight,center}
\begin{tabular}{llrrr}
\hline
 Method        & Dataset                      & RPE transl. [$\frac{m}{s}$]   & RPE rot. [$\frac{\circ}{s}$]  \\% & ATE [m]   \\
\hline
 %Static        & TUM FR2 : desk-with-person   & 0.173               & 9.568         \\%     & 52.608    \\
 %RigidMask     & TUM FR2 : desk-with-person   & 0.066               & 2.872         \\%     & 3.676     \\
 %ORB-SLAM2     & TUM FR2 : desk-with-person   & 0.038               & 1.372         \\%     & 0.006     \\
 %RGBD-SLAM-Dyn & TUM FR2 : desk-with-person   & 0.036               & 1.395         \\%     & 0.008     \\
 %DROSF (ours.) & TUM FR2 : desk-with-person   & 0.043               & 2.616         \\%     & 3.411     \\
 %\hline
 Static        & TUM FR3 : sitting-static     & 0.021               & 4.584         \\%     & 0.792     \\
 RigidMask     & TUM FR3 : sitting-static     & 0.115               & 2.427         \\%     & 6.626     \\
 ORB-SLAM2     & TUM FR3 : sitting-static     & 0.012               & 0.363         \\%     & 0.008     \\
 RGBD-SLAM-Dyn & TUM FR3 : sitting-static     & 0.014               & 0.379         \\%     & 0.010     \\
 \methodname{} (ours.) & TUM FR3 : sitting-static     & 0.047               & 1.637         \\%     & 1.057     \\
  \hline
 Static        & TUM FR3 : sitting-xyz        & 0.165               & 8.632         \\%     & 3.090     \\
 RigidMask     & TUM FR3 : sitting-xyz        & 0.167               & 3.629         \\%     & 9.202     \\
 ORB-SLAM2     & TUM FR3 : sitting-xyz        & 0.014               & 0.582         \\%     & 0.009     \\
 RGBD-SLAM-Dyn & TUM FR3 : sitting-xyz        & 0.013               & 0.579         \\%     & 0.009     \\
 \methodname{} (ours.) & TUM FR3 : sitting-xyz        & 0.110               & 3.137         \\%     & 1.452     \\
  \hline
 Static        & TUM FR3 : sitting-rpy        & 0.059               & 30.647        \\%     & 1.037     \\
 RigidMask     & TUM FR3 : sitting-rpy        & 0.214               & 4.751         \\%     & 7.464     \\
 ORB-SLAM2     & TUM FR3 : sitting-rpy        & 0.038               & 0.936         \\%     & 0.025     \\
 RGBD-SLAM-Dyn & TUM FR3 : sitting-rpy        & 0.032               & 0.905         \\%     & 0.023     \\
 \methodname{} (ours.) & TUM FR3 : sitting-rpy        & 0.128               & 4.078         \\%     & 1.882     \\
  \hline
 Static        & TUM FR3 : sitting-halfsphere & 0.225               & 25.954        \\%     & 3.886     \\
 RigidMask     & TUM FR3 : sitting-halfsphere & 0.184               & 4.522         \\%     & 9.210     \\
 ORB-SLAM2     & TUM FR3 : sitting-halfsphere & 0.037               & 0.910         \\%     & 0.025     \\
 RGBD-SLAM-Dyn & TUM FR3 : sitting-halfsphere & 0.035               & 0.870         \\%     & 0.024     \\
 \methodname{} (ours.) & TUM FR3 : sitting-halfsphere & 0.095               & 3.689         \\%     & 1.728     \\
  \hline 
 Static        & TUM FR3 : walking-static     & 0.020               & 4.431         \\%     & 3.299     \\
 RigidMask     & TUM FR3 : walking-static     & 0.163               & 2.664         \\%     & 9.217     \\
 ORB-SLAM2     & TUM FR3 : walking-static     & 0.583               & 10.576        \\%     & 0.408     \\
 RGBD-SLAM-Dyn & TUM FR3 : walking-static     & 0.014               & 0.329         \\%     & 0.011     \\
 VO-SF         & TUM FR3 : walking-static     & 0.111               & 1.830         \\%     & -         \\
 \methodname{} (ours.) & TUM FR3 : walking-static     & 0.049               & 1.799         \\%     & 1.484     \\
  \hline
 Static        & TUM FR3 : walking-xyz        & 0.265               & 12.397        \\%     & 2.100     \\
 RigidMask     & TUM FR3 : walking-xyz        & 0.284               & 4.400         \\%     & 7.373     \\
 ORB-SLAM2     & TUM FR3 : walking-xyz        & 1.048               & 19.730        \\%     & 0.722     \\
 RGBD-SLAM-Dyn & TUM FR3 : walking-xyz        & 0.127               & 2.741         \\%     & 0.087     \\
 VO-SF         & TUM FR3 : walking-xyz        & 0.304               & 5.69          \\%     & -         \\
 \methodname{} (ours.) & TUM FR3 : walking-xyz        & 0.128               & 3.511         \\%     & 1.020     \\
  \hline
 Static        & TUM FR3 : walking-rpy        & 0.119               & 28.284        \\%     & 3.889     \\
 RigidMask     & TUM FR3 : walking-rpy        & 0.268               & 4.453         \\%     & 9.920     \\
 ORB-SLAM2     & TUM FR3 : walking-rpy        & 1.184               & 22.293        \\%     & 0.805     \\
 RGBD-SLAM-Dyn & TUM FR3 : walking-rpy        & 0.230               & 4.634         \\%     & 0.161     \\
 \methodname{} (ours.) & TUM FR3 : walking-rpy        & 0.165               & 3.872         \\%     & 1.827     \\
  \hline
 Static        & TUM FR3 : walking-halfsphere & 0.281               & 26.313        \\%     & 4.022     \\
 RigidMask     & TUM FR3 : walking-halfsphere & 0.279               & 5.100         \\%     & 9.591     \\
 ORB-SLAM2     & TUM FR3 : walking-halfsphere & 1.079               & 24.663        \\%     & 0.723     \\
 RGBD-SLAM-Dyn & TUM FR3 : walking-halfsphere & 0.052               & 0.985         \\%     & 0.035     \\
 VO-SF         & TUM FR3 : walking-halfsphere & 0.341               & 6.77          \\%    & -         \\
 \methodname{} (ours.) & TUM FR3 : walking-halfsphere & 0.165               & 4.528         \\%     & 1.696     \\
 % \hline
 %Static        & Bonn : balloon-tracking      & 0.252               & 17.394        \\%     & 3.938     \\
 %RigidMask     & Bonn : balloon-tracking      & 0.138               & 4.994         \\%     & 4.432     \\
 %\methodname{} (ours.) & Bonn : balloon-tracking      & 0.101               & 4.367         \\%     & 2.263     \\
 %\hline
 %Static        & Bonn : crowd                 & 0.070               & 9.944         \\%     & 1.820     \\
 %RigidMask     & Bonn : crowd                 & 0.143               & 3.475         \\%     & 7.005     \\
 %\methodname{} (ours.) & Bonn : crowd                 & 0.091               & 3.358         \\%     & 3.327     \\
\hline
\end{tabular}
%\end{adjustbox}

\end{table}

\begin{comment}

\begin{table}[]
\centering
\caption{Odometry evaluation for individual sequences of the Bonn RGB-D dataset based on the relative pose error. For comparison the results of the two-frame based solutions RigidMask \cite{yang2021learning_rigidmask}, VO-SF \cite{jaimez2017fast} and of the model-based solutions RGBD-SLAM-Dyn \cite{dai2020rgb}, ORB-SLAM2 \cite{mur2017orb} are reported if available.}
\label{tab:eval_odo_ate}
%\begin{adjustbox}{totalheight=\textheight,center}
\begin{tabular}{llrrr}
\hline
 Method        & Dataset                      & RPE transl. [$\frac{m}{s}$]   & RPE rot. [$\frac{\circ}{s}$]  \\% & ATE [m]   \\
\hline
 Static        & Bonn : balloon-tracking      & 0.252               & 17.394        \\%     & 3.938     \\
 RigidMask     & Bonn : balloon-tracking      & 0.138               & 4.994         \\%     & 4.432     \\
 \methodname{} (ours.) & Bonn : balloon-tracking      & 0.101               & 4.367         \\%     & 2.263     \\
 \hline
 Static        & Bonn : crowd                 & 0.070               & 9.944         \\%     & 1.820     \\
 RigidMask     & Bonn : crowd                 & 0.143               & 3.475         \\%     & 7.005     \\
 \methodname{} (ours.) & Bonn : crowd                 & 0.091               & 3.358         \\%     & 3.327     \\
\hline
\end{tabular}
%\end{adjustbox}

\end{table}

\end{comment}
