# Supplementary material for: SF2SE3: Clustering Scene Flow into SE(3)-Motions via Proposal and Selection
Source: arXiv:2209.08532 source file (2022-09-26)
Supplement: Supplementary file 2 [file probabilistic_models.tex]

\subsection{Gaussian Inlier Probability}
To calculate the inlier probabilities, we define the inlier probability for a single Gaussian random variable as follows
\begin{gather}
    \label{eq:gauss_inlier_prob}
    P_{I, Gauss.}(a, \mu, \sigma^2) = 2 (1 - F( \mu + |a|, \mu, \sigma^2)) \in [0, 1].
\end{gather}
This is illustrated in Figure \ref{fig:inlier_probab}.
\begin{figure}
    \centering
    \includesvg[scale=0.3]{chapters/3_approach/figures/inlier_probability.svg}
    \caption{On the left side is depicted in blue the probability density function $f(x)$ for a Gaussian distribution with $\mu=0$ and $\sigma^2=1$. The red area indicates the the Gaussian Inlier Probability $P_{I,Gauss}(a=1)$. On the right side, the resulting inlier probabilities are visualized, where the y-axis is shared with the left diagram.}
    \label{fig:inlier_probab}
\end{figure}
